# Supplementary material for: Stochastic Frank-Wolfe for Constrained Finite-Sum Minimization
Source: arXiv:2002.11860 source file (2022-09-08)
Supplement: Supplementary file 1 [file appendix_SAGA_variant.tex]

\begin{algorithm}[hb]
   \caption{Stochastic Frank-Wolfe - SAGA variant} \label{alg:sfw_saga}
\begin{algorithmic}[1]
   \STATE {\bfseries Initialization:} $\ww_0\in\CC$, $\balpha_0 \in \RR^n$, ${\rr_0 =\XX^\top\balpha_0}$
%   \STATE Use step size $\gamma_t=2/(t+2)$.

    \FOR{$t=1, 2, \dots, $}
        \STATE Sample $i \in \{1, \ldots, n\}$ uniformly at random. \label{lst:line:sample}
        \STATE Update $\balpha_t^i = \frac{1}{n}f'_i(\xx_i\tran\ww_{t-1})$ \label{lst:line:refresh_alpha}
       
        \STATE $\rr_{t} = \rr_{t-1} + (\balpha_{t}^i - \balpha_{t-1}^i) \xx_i$ \label{lst:line:refresh_gradient}
    
        \STATE $\sss_t = \LMO(\rr_t + (n-1)(\balpha_t^i - \balpha_{t-1}^i)\xx_i)$  \label{lst:line:lmo}
        
        \STATE $\ww_{t} = \ww_{t-1} + \frac{2}{t+2}(\sss_t - \ww_{t-1})$  \label{lst:line:update_iterate}
   \ENDFOR
\end{algorithmic}
\end{algorithm}

We define a SAGA analog for FW, see Algorithm~\ref{alg:sfw_saga}. In this variant, the gradient estimator we use as argument to the LMO is: $\bbeta_t = \balpha_t + (n-1)(\balpha_t^i - \balpha_{t-1}^i)\ee_i$. We define $H_t$ as the $\ell_1$ error between this estimator and the true gradient at $\XX\ww_{t-1}$:

\begin{align}
    H_t &= \|\bbeta_t - \nabla f(\XX\ww_{t-1})\|_1.
\end{align}

Now, as for the SAG variant, we want to bound the conditional expectation of $H_t$. The randomness is that of the choice of $i$ at step $t$.

\begin{align}
    \EE_t H_t &= \EE_t\|\balpha_t + (n-1)(\balpha_t^i - \balpha_{t-1}^i)\ee_i - \nabla f(\XX\ww_{t-1})\|_1 \\
    &= \EE_t \|\balpha_{t-1} + n(\balpha_t^i - \balpha_{t-1}^i)\ee_i - \nabla f(\XX\ww_{t-1})\|_1
\end{align}

Let us examine this coordinate wise. Coordinate $j$ is selected with probability $\frac{1}{n}$, therefore:

\begin{align}
    \EE_t |\bbeta_t^j - \frac{1}{n} f'_j(\xx_j\tran\ww_{t-1})| &= \EE_t\left|\balpha_{t-1}^j + n(\balpha_t^i - \balpha_{t-1}^i)\one_{i=j} - \frac{1}{n} f'_j(\xx_j\tran\ww_{t-1})\right| \\
    &= \left(1-\frac{1}{n}\right)\left|\balpha_{t-1}^j - \frac{1}{n}f'_j(\xx_j\tran\ww_{t-1})\right| + \frac{1}{n}\left|\frac{n-1}{n}f'_j(\xx_j\tran\ww_{t-1})-(n-1)\balpha_{t-1}^j \right| \\
    &= 2 \left(1-\frac{1}{n}\right) \left|\balpha_{t-1}^j - \frac{1}{n}f'_j(\xx_j\tran\ww_{t-1})\right| 
\end{align}

Meaning that the conditional expectation of $H_t$ is:

\begin{align}
    \EE_t H_t = 2 \left(1-\frac{1}{n}\right) \|\balpha_{t-1}^j - \nabla f(\XX\ww_{t-1})\|_1.
\end{align}
 
This is exactly twice the value for the SAG variant. The rest of the proof therefore works in the same way, giving the same overall rate (apart from the introduced factor of 2).
