# Supplementary material for: Stochastic Frank-Wolfe for Constrained Finite-Sum Minimization
Source: arXiv:2002.11860 source file (2022-09-08)
Supplement: Supplementary file 2 [file appendix_almost_sure_convergence.tex]

We want to show almost sure convergence of our algorithm to an optimum, in the convex case at least.

Let us base our thoughts on the following Lemma, from Bertsekas, and reported in \citet{mokhtari2018stochastic} (page 29).

\begin{lemma}
Let $\{X_t\}$, $\{Y_t\}$, $\{Z_t\}$ be three sequences such that $Y_t \geq 0$ for all $t$. Suppose that for all $t$,
\begin{align}
    X_{t+1} \leq X_t - Y_t + Z_t
\end{align}
and that $\sum_{t=0}^\infty Z_t < \infty$. Then, either $X_t \to -\infty$ or $\{X_t\}$ has a finite limit, and $\sum_{t=0}^\infty Y_t < \infty$.
\end{lemma}

Recall that from Lemma 1 (which assumes convexity of the objective), we have the following bound on the suboptimality $\varepsilon_t$

\begin{align}
    \varepsilon_t \leq (1-\gamma_t) \varepsilon_{t-1} + \gamma_t D_\infty H_t + \gamma_t^2\frac{ L D_2^2}{2n}.
\end{align}

We would like to use the previous lemma, with $X_t = \varepsilon_t$, $Y_t = \gamma_t \varepsilon_t$ and $Z_t =\gamma_t D_\infty H_t + \gamma_t^2\frac{ L D_2^2}{2n}$. Since $\varepsilon_t \geq 0$ for all $t$, the second case would apply. Then $\gamma_t \varepsilon_t$ would be summable, which implies almost-sure convergence of $\varepsilon_t$ to 0.

The second term in this $Z_t$ is summable, therefore, we only need to show that $\gamma_t H_t$ is almost surely summable.

Using Young's inequality, we have for any $\beta_t$,

\begin{align}
    \gamma_t H_t \leq  \frac{\gamma_t^2}{\beta_t} + \beta_t H_t^2. 
\end{align}

Using this, we would only need to choose $\beta_t$ such that $\gamma_t^2 / \beta_t$ and $\beta_t H_t^2$ are summable. 

Our Lemma \ref{lemma:ht_upper_bound} suggests possible super-martingale behavior, and that $H_t$ is an easier quantity to study than $H_t^2$, since we have this inequality

\begin{align}
    \EE_t H_t \leq \rho\left( H_{t-1} + \gamma_{t-1} \frac{LD_1}{n}\right),
\end{align}
where $\rho = 1 - \frac{k}{n}$, where $k$ is our batch size, and $n$ the total number of samples.

From \citet{mokhtari2018stochastic}, it seems that a sufficient result would be the existence of non-negative random variables $\zeta_t$ and $\xi_t$ such that:

\begin{align}
    \EE_t \zeta_t \leq \zeta_{t-1} - \xi_{t-1}.
\end{align}

Then, using a result on super martingale convergence, we would get that $\xi_t$ is almost surely summable. It would make sense that $\xi_t$ would be proportional to $\gamma_t H_t$, or perhaps to $H_t$ itself, which would give the stronger result that $\sum_t H_t < \infty$.

One idea is to split the bound on $\EE_t H_t$:

\begin{align}
    \EE_t H_t \leq H_{t-1} - \frac{k}{n}H_{t-1} + \rho\gamma_{t-1} \frac{LD_1}{n}.
\end{align}

Following the method in \citet{mokhtari2018stochastic}, it almost seems like we could use $\xi_t = \frac{k}{n}H_{t}$, and $\zeta_t = H_t + \frac{LD_1}{n} \rho \sum_{s=t+1}^\infty \gamma_s $, but this isn't defined for $\gamma_t = \frac{2}{t+2}$. Another attempt would be to use:
\begin{align}
   \zeta_t = H_t + \frac{LD_1}{n} \rho \sum_{s=t}^\infty \rho^{s-t}\gamma_s,
\end{align}
but then

\begin{align}
    \EE_t [\zeta_t] - \zeta_{t-1} \leq -\frac{k}{n} H_{t-1} + \frac{LD_1}{n} (1-\rho) \sum_{s=t}^\infty \rho^{s-t}\gamma_s,
\end{align}
which isn't guaranteed to be negative, even after a while... It seems like this is really close to something we would want.
