# Supplementary material for: Stochastic Frank-Wolfe for Constrained Finite-Sum Minimization
Source: arXiv:2002.11860 source file (2022-09-08)
Supplement: Supplementary file 3 [file appendix_full_gradient_comparison.tex]

We derive the rate for the full gradient, deterministic Frank-Wolfe in the finite sum setting, to make comparison with our method easier.

Let us first write the Frank-Wolfe algorithm, using our notations.

\begin{algorithm}[hb]
  \caption{Frank-Wolfe algorithm \cite{frank1956algorithm}}
  \label{alg:fw}
\begin{algorithmic}
  \STATE {\bfseries Initialization:} $\ww_0\in\CC$
    \FOR{$t=1, 2, \dots, $}

        \STATE $\balpha_t = \nabla f(\XX\ww_{t-1})$
        \STATE $\rr_t = \XX\tran \balpha_t$
        \STATE $\sss_{t} = \LMO(\rr_t)$\\
        \STATE $\ww_{t} = (1 - \gamma_t)\ww_{t-1} + \gamma_t \sss_t$ 
  \ENDFOR
\end{algorithmic}
\end{algorithm}

% We are optimizing the main equation \eqref{eq:obj_fun}. 
% For all $\ww$, $f(\XX\ww) = \frac{1}{n}\sum_{i=1}^nf_i(\xx_i\tran \ww)$. We suppose each $f_i$ is $L$-smooth and convex. Let $\varepsilon_t = f(\XX\ww_t) - f(\XX\ww_\star)$ be the primal suboptimality at step t.

% Under these hypotheses, Lemma \ref{lemma:sufficient_decrease} applied with $\balpha_t = \nabla f(\XX\ww_{t-1})$ (and therefore $H_t = 0$) allows us to bound the primal suboptimality as follows:

% \begin{align}
%     \epsilon_t \leq (1-\gamma_t)\epsilon_{t-1} + \gamma_t^2 \frac{LD^2_2}{2n}.
% \end{align}

% Then using the step size $\gamma_t = \frac{2}{t+2}$, defining $\Gamma_t = (t+1)(t+2) \varepsilon_t$ and upper bounding $\frac{t+1}{t+2}$ by $1$, we get

% \begin{align}
%     \Gamma_t \leq \Gamma_{t-1} + 2\frac{LD_2^2}{n}.
% \end{align}

% Summing over iterations from $k=1,\dots, t$, we get

% \begin{align}
%     \Gamma_t \leq \Gamma_{0} + 2t\frac{LD_2^2}{n}.
% \end{align}

% Dividing back by $(t+1)(t+2)$ and using the bound $\frac{1}{(t+1)(t+2)} \leq \frac{1}{t^2}$, we get the usual Frank-Wolfe rate:

% \begin{align}
%     \varepsilon_t \leq  2\frac{LD_2^2}{nt} + \frac{\varepsilon_0}{t^2}
% \end{align}

% By using $\balpha_0=0$ and setting $\ww_{-1}$ as our initial iterate, we can remove the $\frac{\varepsilon_0}{t^2}$ term, and only obtain $\frac{2LD_2^2}{t}$ as in \citet{jaggi2013revisiting, lacoste2015global}.

\subsection{Comparison w.r.t. gradient calls.}

In the full gradient setting, one iteration makes $n$ gradient calls. Therefore, if $u=nt$ is the number of gradient calls after $t$ iterations, we obtain the following bound in the full gradient case, using the slight abuse of notation $\epsilon_u$ to denote the suboptimality after $u$ gradient calls.

\begin{align}
    \varepsilon_u \leq  \frac{2LD_2^2}{u}.
\end{align}

Compare to our method, after $t$ iterations (and therefore after $t$ gradient calls), as shown in Theorem \ref{theorem:convex_rate}

\begin{align}
\bsp
    \EE\varepsilon_t \leq& 2L\left( \frac{D^2_2 + 4(n-1)D_1D_\infty}{n}  \right) \frac{t}{(t+1)(t+2)} \\
    &+  \frac{2 \varepsilon_0 + (2 D_\infty H_0 + 64 {L D_1 D_\infty}) n^2}{(t+1)(t+2)}
\esp
\end{align}

\pagebreak
