# Supplementary material for: Stochastic Frank-Wolfe for Constrained Finite-Sum Minimization
Source: arXiv:2002.11860 source file (2022-09-08)
Supplement: Supplementary file 4 [file appendix_primal_dual.tex]

\section{Primal-Dual proof}

Define $\bmu_t = (1-\gamma_t)\bmu + \balpha_t$. Let $\psi$ be the negative dual function.

Then,

\begin{align}
    f(\XX\ww_t) &\leq f(\XX\ww_{t-1}) - \gamma_t \langle \nabla f(\XX\ww_{t-1}), \ww_{t-1} - \sss_t\rangle + \gamma_t^2 \frac{LR^2}{2} \\
    &\leq f(\XX\ww_{t-1}) - \gamma_t \hat{g}_t + \langle \nabla f(\XX\ww_{t-1}) - \balpha_t, \ww_{t-1} - \sss_t\rangle + \gamma_t^2 \frac{LR^2}{2}
\end{align}

Remark that
\begin{align}
    \hat{g}_t = f(\XX\ww_{t-1}) + \psi(\balpha_t) - \Delta_\ast(\nabla f(\XX\ww_{t-1}), \balpha_t)
\end{align}

where $\Delta_\ast(\balpha, \bbeta) = f^\ast(\balpha) - f^\ast(\bbeta) - \langle \nabla f^\ast(\bbeta), \balpha-\bbeta\rangle$ is the Bregman divergence of the strongly-convex function $f^\ast$.

Plugging this back, we get:

\begin{align}
    f(\XX\ww_t) &\leq  (1-\gamma_t)f(\XX\ww_{t-1}) - \gamma_t\psi(\balpha_t) + \gamma_t \Delta_\ast(\nabla f(\XX\ww_{t-1}), \balpha_t) + \gamma_tR_2 H_t + \gamma_t^2 \frac{LR^2}{2}
\end{align}

Now, since $\psi$ is convex, the following inequality holds: $\psi(\bmu_t) \leq (1-\gamma_t)\psi(\bmu_{t-1}) + \gamma_t \psi(\balpha_t)$, and therefore,

\begin{align}
    f(\XX\ww_t)+ \psi(\bmu_t) &\leq  (1-\gamma_t)\left(f(\XX\ww_{t-1}) - \psi(\bmu_{t-1})\right) + \gamma_t \Delta_\ast(\nabla f(\XX\ww_{t-1}), \balpha_t) + \gamma_tR_2 H_t + \gamma_t^2 \frac{LR^2}{2}
\end{align}

Generalized triangle inequality: $\forall \balpha, \bbeta, \bmu$,

\begin{align}
    \Delta_\ast(\balpha, \bbeta) + \Delta_\ast(\bbeta, \bmu) = \Delta_\ast(\balpha, \bmu) + \langle \balpha - \bbeta, \nabla f^\ast(\bmu) - \nabla f^\ast(\bbeta) \rangle
\end{align}

Perhaps use this for Lyapunov of the form

\begin{align}
    f(\XX\ww_t)+ \psi(\bmu_t) + c \Delta_\ast(\nabla f(\XX\ww_{t}), \balpha_{t+1})
\end{align}

??
