# Supplementary material for: Stochastic Frank-Wolfe for Constrained Finite-Sum Minimization
Source: arXiv:2002.11860 source file (2022-09-08)
Supplement: Supplementary file 5 [file appendix_standalone_proof_corrected_05052020.tex]

\subsection{Hypotheses}

We want to prove the convergence rate of algorithm~\ref{alg:stochasticfw} on a problem of the form~\ref{eq:fw_objective}.

We suppose that $f(\btheta) = \frac{1}{n}\sum_i f_i(\btheta^i)$, and that our full objective is:

\begin{align}
    \min_{\ww\in\CC} f(\XX\ww).
\end{align}

We additionally suppose that the $f_i$ are convex and $L$-smooth, yielding that $f$ is  $(L/n)$-smooth with respect to the $\ell_2$ norm as per \eqref{norman}.

Let us define the quantities $D_p = \max_{\ww \in \CC - \CC} \|Xw\|_p$. These are a kind of diameters attached to the $\ell_p$ norms.

\subsection{Proof}

The proof of Lemma ~\ref{lemma:sufficient_decrease} in Appendix~\ref{apx:sufficient_decrease} is correct. Under the previous hypotheses, we get the following upper bound on the suboptimality:

\begin{align}
\bsp
    \varepsilon_t  \leq~&  (1-\gamma_t)\varepsilon_{t-1} + \gamma_t^2\frac{LD^2_2}{2n}+ \gamma_t D_\infty H_t,
\esp
\end{align}

where $\varepsilon_t = f(\XX\ww_t) - f(\XX\ww_\star)$, $H_t = \|\balpha_t - \nabla f(\XX\ww_{t-1})\|_1$ and $D = \max_{\uu,\vv\in \CC}\|\XX(\uu-\vv)\|_{\infty}$.

\textbf{See Appendix~\ref{apx:sufficient_decrease}.}

The proof of Lemma~\ref{lemma:ht_upperbound} is also correct {\blue strange thing to say + broken link} that's a, yielding the following upper bound for $\EE_t H_t$ (the conditional expectation of $H_t$):

\begin{align}
    \EE_t H_t \leq \left(1-\frac{1}{n}\right)(H_{t-1} + \gamma_{t-1}LD).
\end{align}

\textbf{See in main text.}

On the other hand, the statement and proof of Lemma~\ref{lemma:ht_asymptotics} were incorrect. The corrected version follows.

\input{lemma_3_fix}

\textbf{Tying everything together.}

\input{appendix_tying_up}
